# Supplementary material for: Understanding correlations in BaZrO3:Structure and dynamics on the nano-scale
Source: arXiv:2310.05565 ancillary file (2023-10-09)
Supplement: Supplementary file 1 [file supp.pdf]

# Supporting Information:

# Understanding correlations in $BaZrO_3$: Structure and dynamics on the nano-scale

Erik Fransson[1], Petter Rosander[1], Paul Erhart[1], and Göran Wahnström[1]

[1] *Department of Physics, Chalmers University of Technology, SE-41296, Gothenburg, Sweden*

October 6, 2023

# Contents

**Training of the NEP potential** **2**

**Validation of the NEP potential** **4**

**Motivation for the employed exchange-correlation functional** **6**

**Thermal expansion** **7**

**Quantum effects** **8**

**The electron atomic scattering factor** **10**

**Scattering intensity** **11**

**Static tilt angle correlations** **12**

**Dynamic tilt angle correlations** **13**

**Supplemental References** **14**

# Training of the NEP potential

A neuroevolution potential (NEP) model was fitted with the GPUMD package (version 3.5)[1,2]. The NEP is based on a neural network for which local atomic environments are described by descriptors defined in Ref. 3, here with radial and angular cutoff of 8 Å and 4 Å, respectively, and radial and angular order 8 and 6, respectively. The neural network consists of one hidden layer of 50 neurons and a hyperbolic tangent activation function and was trained over 300 000 generations using the natural evolution strategy[4] implemented in GPUMD. Both the $L_1$ and the $L_2$ norm were regularized using $\lambda_1 = \lambda_2 = 0.1$ (as defined in Ref 2). The model was fitted to forces, energies and virials from density functional theory (DFT) calculation of 655 atomic structures.

The training structures from molecular dynamics (MD) were generated with an active learning scheme as done in Ref. 5. First, 25 models were trained on random splits of the initial training set. Next, MD simulations were run at various temperatures and pressure and for each snapshot the uncertainty in energy (and forces) were evaluated by computing the standard deviation over the predicted energies using the 25 models. The snapshot for each MD simulation with the largest energy uncertainty was selected as a new training structure. This is illustrated for a single trajectory in Fig. S1.

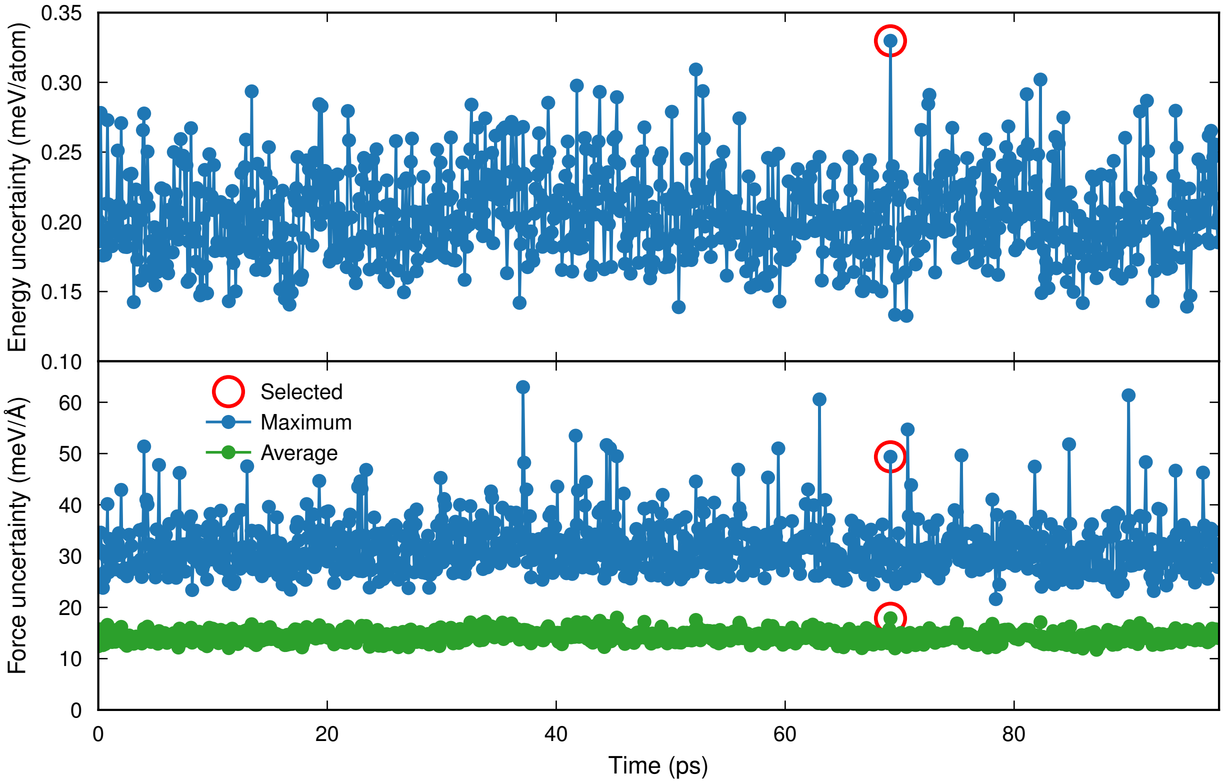


Figure S1: Structure selection for training the NEP via energy uncertainty quantification for a MD trajectory at 500 K. Here the average and maximum uncertainty for the forces is also showed as reference. The selected structure to be added to the training set is marked with the red circle.

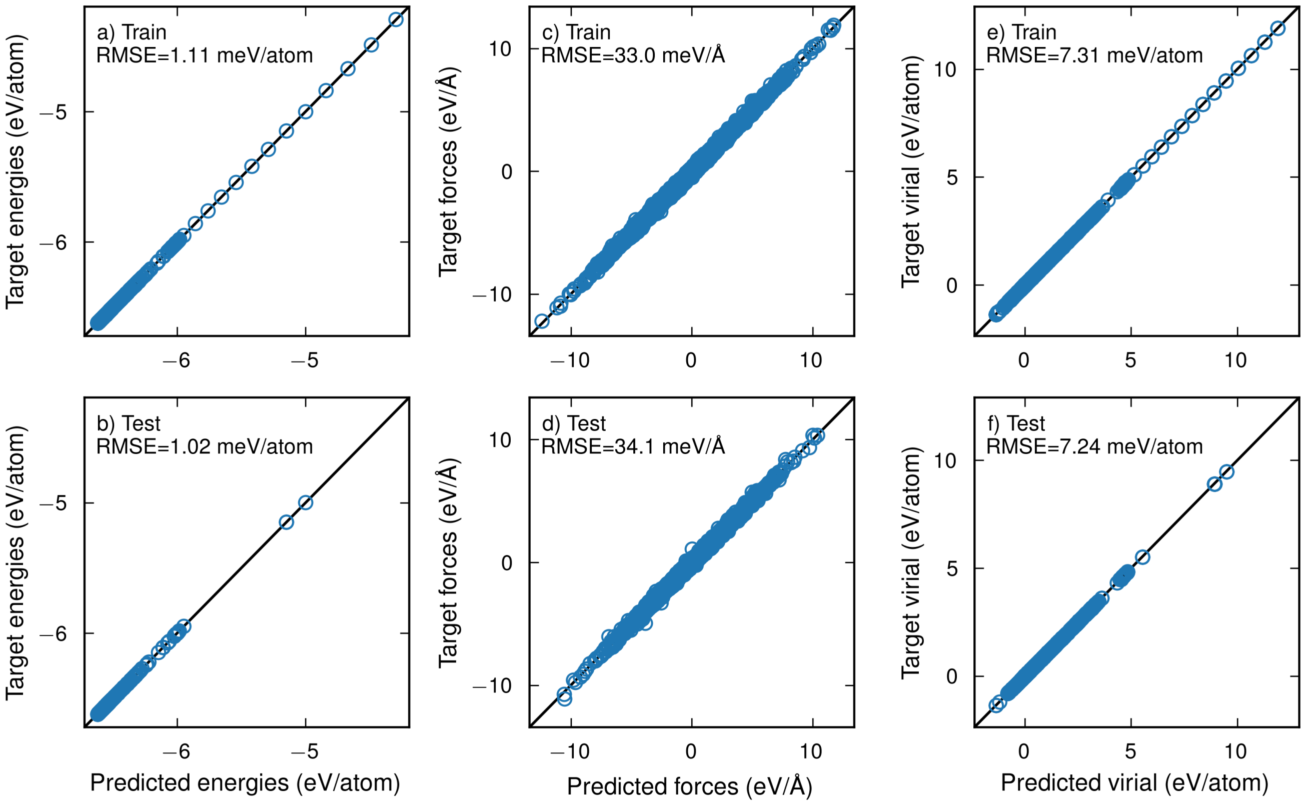


Figure S2: Parity plots for total energies, forces and virials for training and test set.

## Validation of the NEP potential

Here we validate the NEP potential by comparing with DFT results for the energies of various structures and the phonon dispersion curves for the cubic phase. The energy for NEP and DFT has separately been shifted such that the energy is zero for the cubic structure at 4.20 Å.

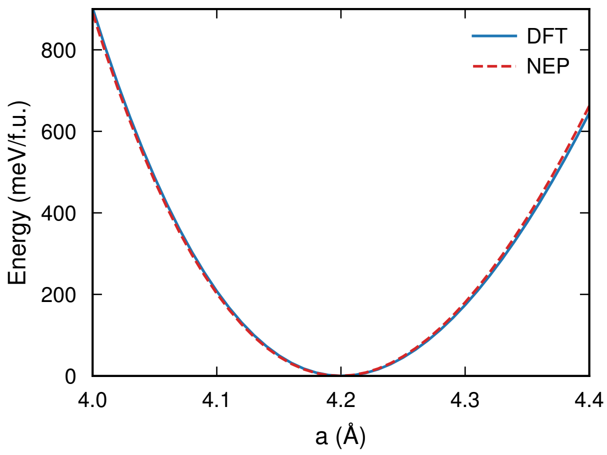


Figure S3: Equation of state for the cubic phase with both DFT and NEP. The NEP model agrees very well with the DFT data. At 4.00 Å the energy for NEP is only 11 meV/f.u. below the DFT value.

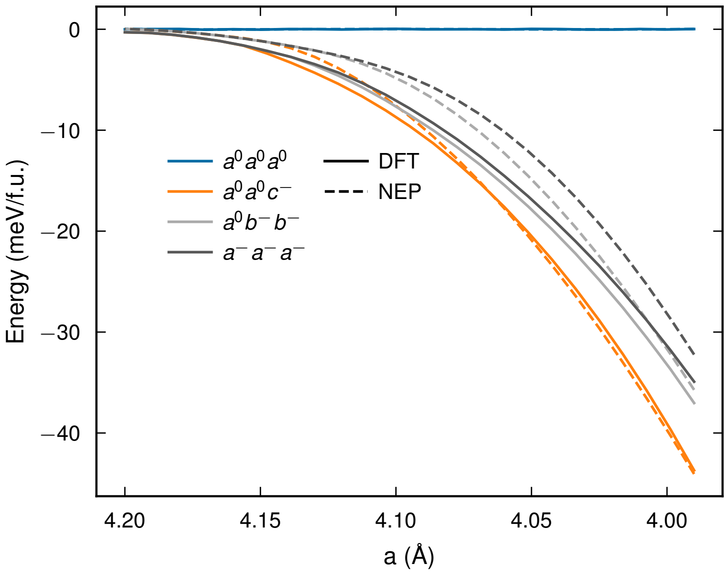


Figure S4: Calculated DFT and NEP energies for the cubic $Pm\bar{3}m$ ($a^0a^0a^0$), tetragonal $I4/mcm$ ($a^0a^0c^-$), orthorhombic $Pnma$ ($a^0b^-b^-$), and rhombohedral $R\bar{3}c$ ($a^-a^-a^-$) structures. The structures are relaxed with NEP and then these structures are used without further relaxation in the DFT evaluation. The cubic structure for NEP and DFT, respectively, are taken as a reference at each lattice parameter. For the non-cubic structures the lattice parameter a refers to the effective cubic lattice parameter $V^{1/3}$.

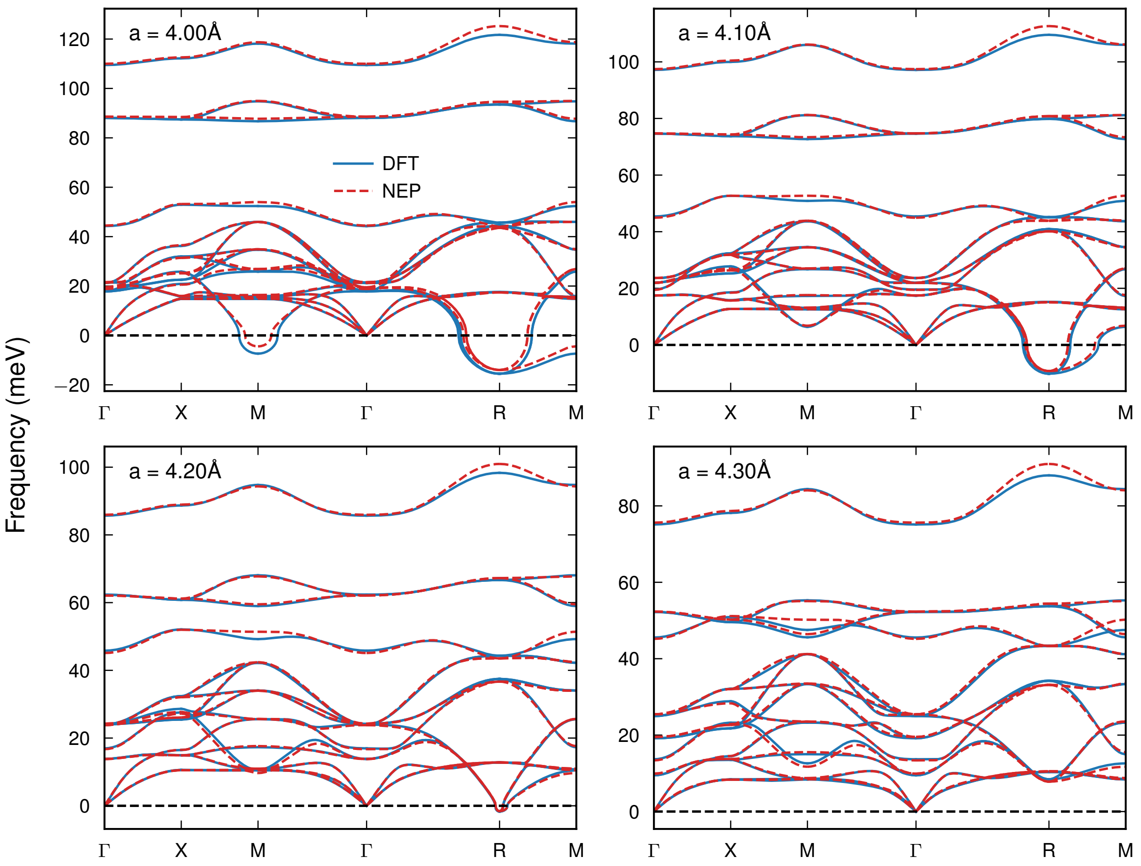


Figure S5: Phonon dispersion for the cubic phase calculated with PHONOPY[6], where solid lines show the results using DFT and dashed lines using NEP.

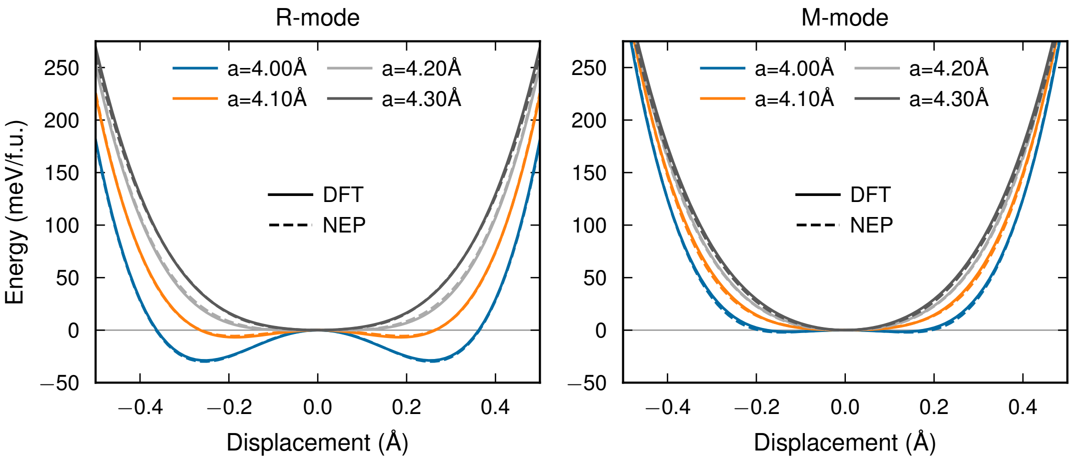


Figure S6: The potential energy surface for the out of phase (R) - and in phase (M) tilt modes at different lattice parameters. Here, solid lines corresponds to DFT calculations and dashed lines to NEP.

# Motivation for the employed exchange-correlation functional

**Harmonic frequencies** In Table S1 theoretical data for the harmonic frequencies at the Γ-point in units of meV are compared with experimental data. The PBE functional underestimates consistently the frequencies. The three functionals PBEsol, WC and CX improve substantially on PBE and the computational cost for these three are very similar as for PBE. Two of the hybrid functionals CX0p and PBE0 improve on the frequencies, but the increase in computational cost is substantial.

| Mode | PBE | PBEsol | WC | CX | PBE0 | HSE | CX0p | Exp. |
|---|---|---|---|---|---|---|---|---|
| TO1 | 11.7 | 12.5 | 11.9 | 13.4 | 16.0 | 13.1 | 14.6 | 14.4 (116) |
| LO1 | 15.4 | 16.5 | 16.5 | 16.6 | 18.1 | 16.6 | 17.6 | 17.5 (141) |
| TO2 | 22.1 | 23.6 | 23.9 | 23.8 | 27.0 | 24.9 | 25.9 | 26.5 (214) |
| LO2 | 45.8 | 45.4 | 45.4 | 45.7 | 49.2 | 48.9 | 48.5 | 47.1 (380) |
| TO3 | 57.1 | 61.7 | 62.4 | 61.2 | 63.1 | 60.2 | 63.2 | 64.5 (520) |
| LO3 | 81.7 | 85.2 | 85.8 | 84.7 | 83.9 | 85.0 | 87.5 | 85.8 (692) |
| error | 3.7 | 1.8 | 1.7 | 1.7 | 1.3 | 1.8 | 0.9 | |

Table S1: Theoretical and experimental data for the phonon frequencies at the Γ-point for $BaZrO_3$ in meV. The PBE, CX, HSE and CX0p data are taken from Ref. 7, the PBEsol from Ref. 8, the WC data from Ref. 9, and the PBE0 data from Ref. 10. Experimental data ($cm^{-1}$, in parentheses) are from Nuzhnyy *et al.*[11], analyzed in Ref. 9. The indicated errors are the average absolute value of the deviation between the theoretical and experimental numbers.

**Anharmonicity** The treatment of anharmonicity, and in particular the temperature dependence of the R-tilt mode is important. The temperature dependent frequency of the R-tilt mode obtained from self-consistent phonon (SCP) (with classical statistics) is shown in Fig. S7 using PBE, PBEsol or CX, and are all consistent with the experimental result in Ref. 12. For explanation of the present SCP method, see Ref. 12.

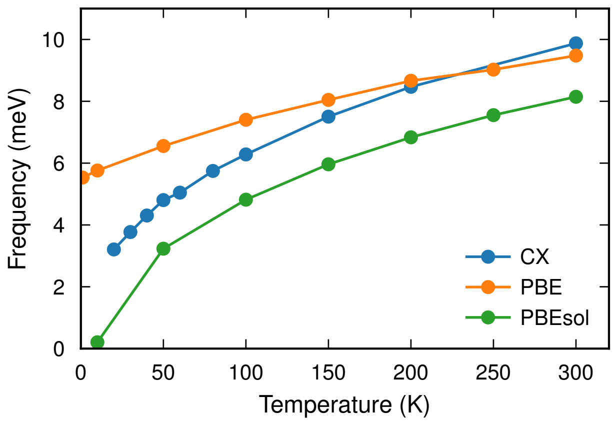


Figure S7: The obtained frequency of the R tilt-mode using SCP with classical statistics. Here, the CX data is from the present study and the PBE and PBEsol data is from Ref. 12.

**Thermal expansion** In Ref. 7 it was found that the thermal expansion of $BaZrO_3$ is considerably better described by CX compared with PBE.

To conclude, the CX functional gives an accurate description of the vibrational motion, including anharmonicities and thermal expansion for $BaZrO_3$, at a computational cost similar to PBE.

## Thermal expansion

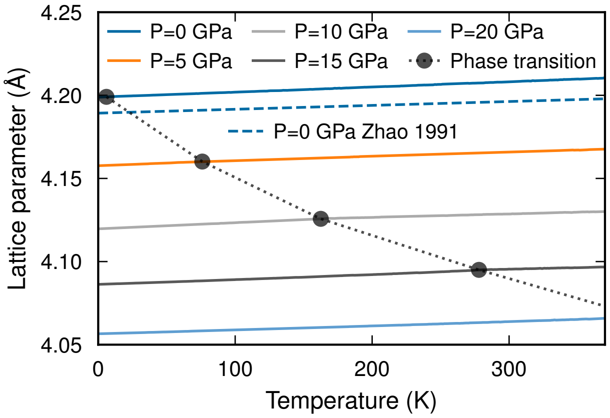


Figure S8: The effective lattice parameter, calculated from $V^{1/3}$, as a function of temperature for a few different pressures. The dashed line corresponds to experimental data obtained via XRD from Ref. 13. The dotted lines with filled circles indicate where the phase transitions between tetragonal and cubic is for each pressure.

# Quantum effects

In order to understand the quantum effects (compared to classical sampling in MD) we employ a self-consistent phonon approach (SCP) using HIPHIVE[14]. This is done in the same way as done in Ref. 12, but using the NEP as the anharmonic potential rather than higher order force constants. The obtained temperature dependency of the R tilt-mode is shown in Fig. S9. Here, the results from peak fitting $S(\boldsymbol{q}, \omega)$ are also included.

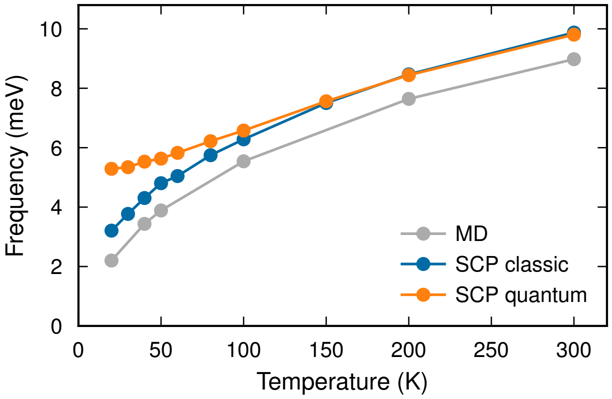


Figure S9: The obtained frequency of the R tilt-mode using MD and SCP. The SCP is carried out using both classical and quantum statistics (see Ref. 12 for more details). This is done with the NEP based on CX.

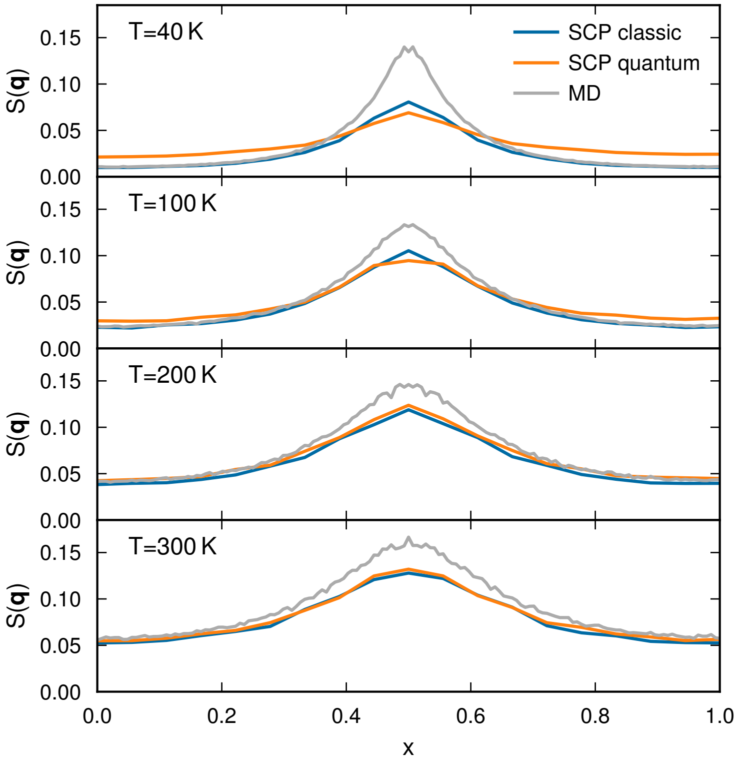


Figure S10: The obtained structure factor, $S(\boldsymbol{q})$, along the M - R - M path using MD and SCP. The SCP is carried out using both classical and quantum statistics. Note that SCP overestimates the R-tilt mode frequency compared to MD (see Fig. S9). Here, $\boldsymbol{q} = \frac{2\pi}{a}(3/2, 1/2, x)$, which corresponds to a path from an M-point ($x$=0), passing an R-point ($x$=1/2) and ending at an M-point ($x$=1). For explanation of the present SCP method, see Ref. 12.

## The electron atomic scattering factor

In the paper the electron atomic scattering factors for the ions are used. The considered 1D slice in $q$-space, from M through R to M ($\boldsymbol{q} = \frac{2\pi}{a}(3/2, 1/2, x)$, where $x$ goes from 0 to 1), corresponds to $s$ changing from 0.19 Å$^{-1}$ to 0.22 Å$^{-1}$. As seen in the figure, the factors for the neutral atoms and the corresponding ions are very similar for those $s$-values.

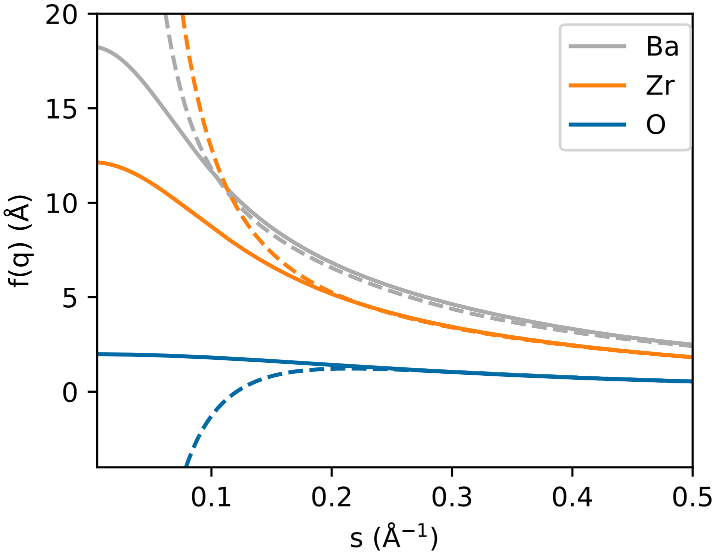


Figure S11: Electron atomic scattering factors for the neutral atoms (solid lines) and the corresponding ions $Ba^{2+}$, $Zr^{4+}$ and $O^{2-}$ (dashed lines) as function of $s$, where $q = 4\pi s$. The data for the neutral atoms and the ions are taken from Refs 15 and 16, respectively.

# Scattering intensity

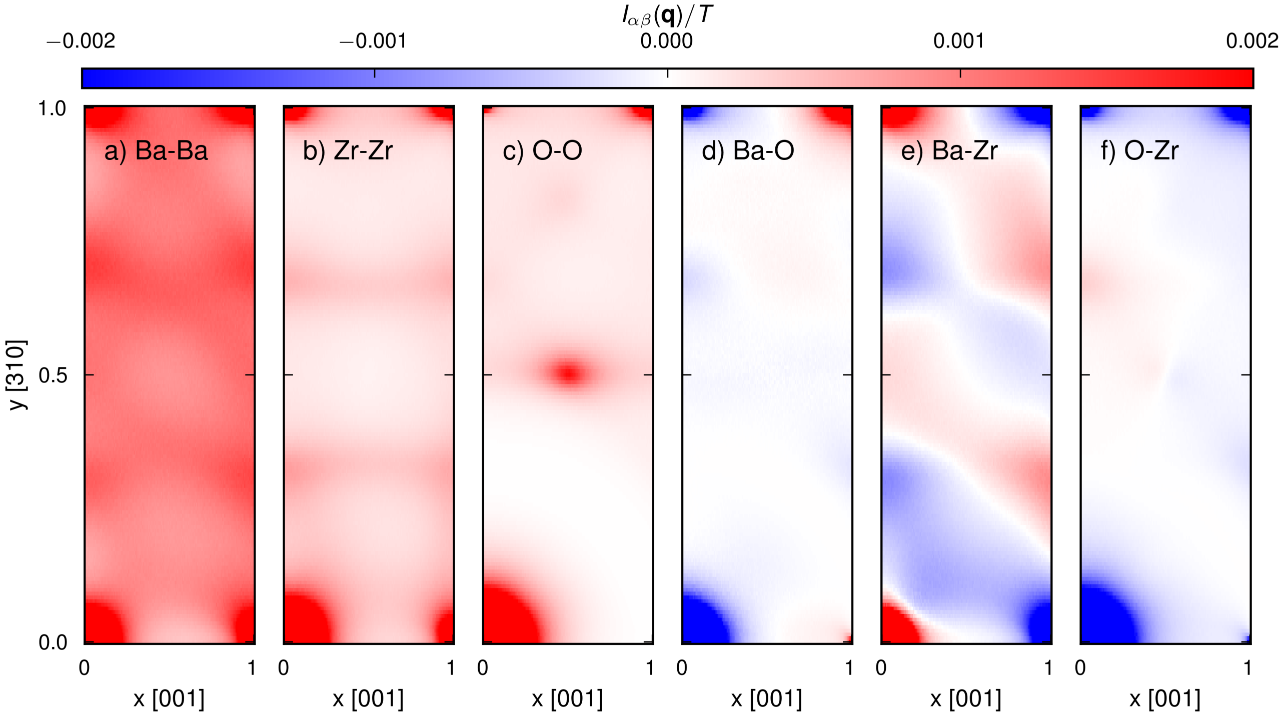


Figure S12: The partial intensity $I_{\alpha\beta}(\boldsymbol{q})$ at 100 K and 0 GPa. Note that cross terms, $\alpha \neq \beta$, are defined with a factor two to account for the symmetry $I_{\alpha\beta}(\boldsymbol{q}) = I_{\beta\alpha}(\boldsymbol{q})$, meaning that the sum over these six heatmaps yields the total intensity $I(\boldsymbol{q})$.

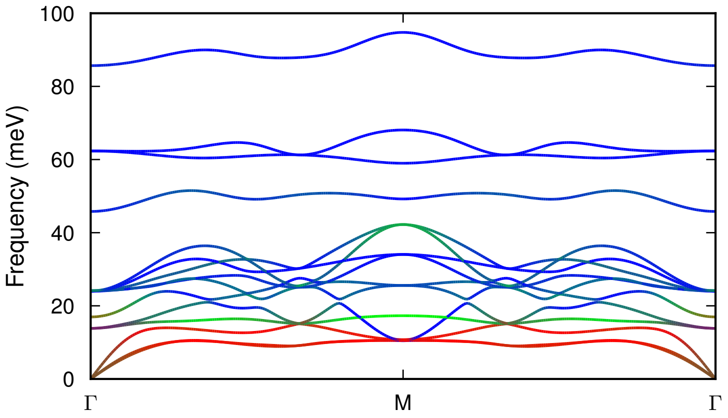


Figure S13: Harmonic phonon dispersion along the path [0, 0, 1] to [3, 1, 1] at a lattice parameter of 4.2 Å. The harmonic force-constants are obtained with DFT using PHONOPY[6]. The color in RGB corresponds to the participation ratio between Ba (red), Zr (green) and O (blue).

## Static tilt angle correlations

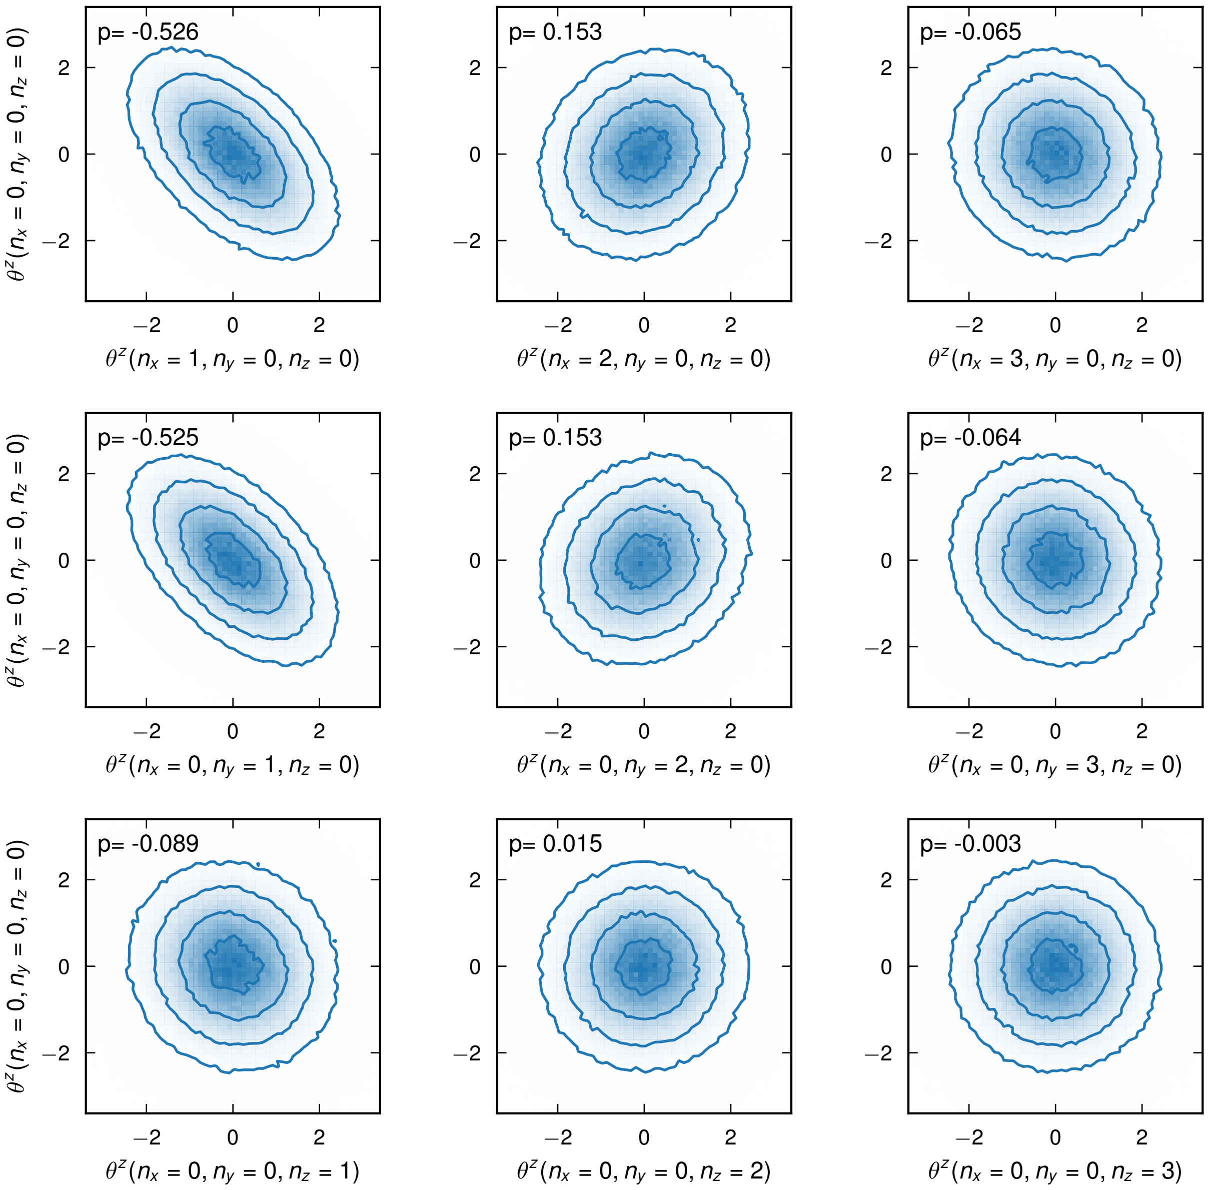


Figure S14: Joint probability distribution over the tilt-angles, $\theta^z$ for neighboring octahedra at T=100 K and P=0 GPa. Here all angels are consider at the same time $t$ and given degrees and p is the correlation coefficient for each neighbor pair. Note that for $\theta^z$ the correlation is stronger for neighbors in the [100] and [010] directions (corresponding to $G_\perp$), whereas the correlation is weaker for neighbors in the [001] direction (corresponding to $G_\parallel$).

## Dynamic tilt angle correlations

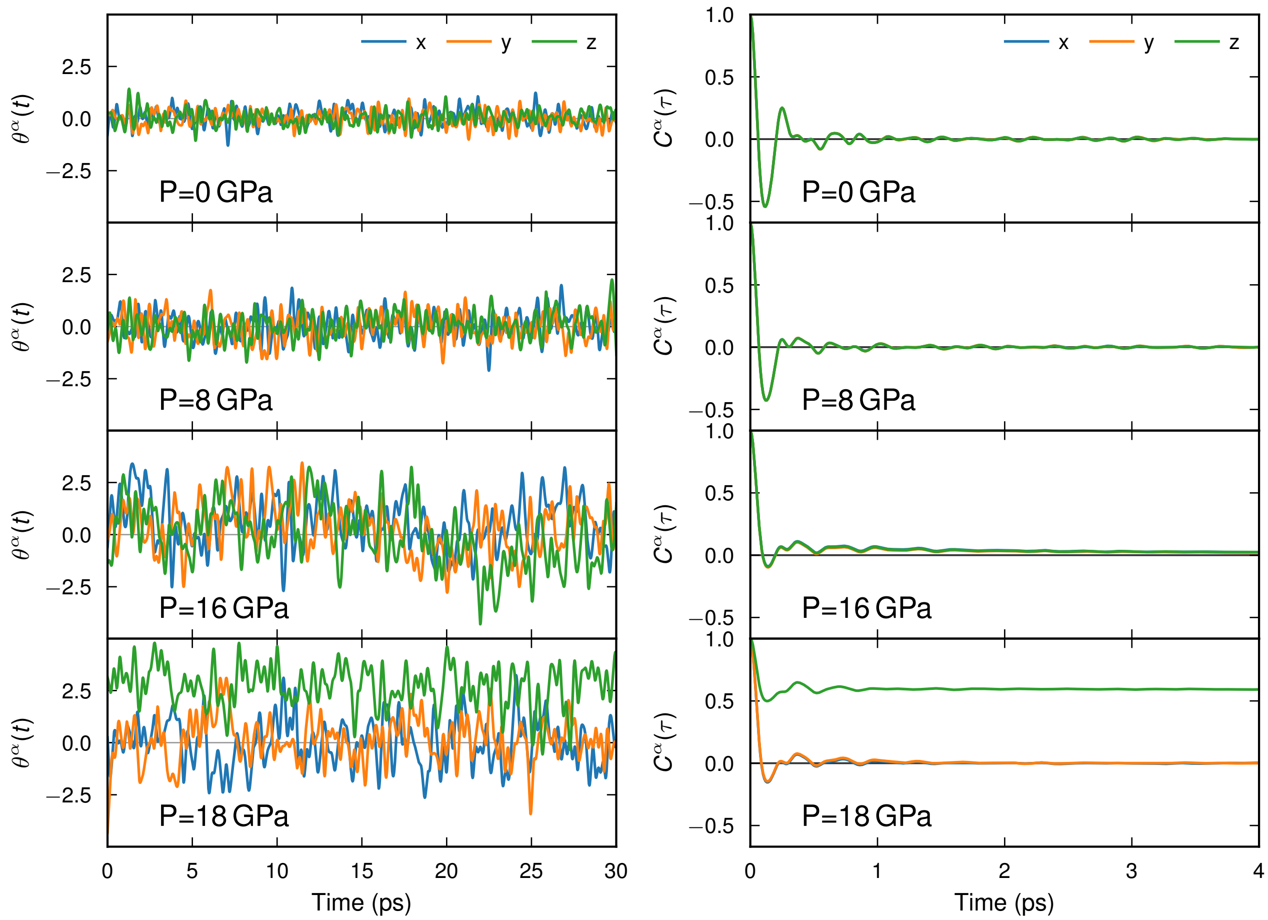


Figure S15: Tilt angles, $\theta^\alpha(t)$, for a single octahedron as a function of time (left), and their corresponding autocorrelation functions, $C^\alpha(\tau)$, averaged over all octahedra (right) at T=300 K. Here, $\theta^\alpha(t)$ is averaged in time over 0.5 ps with a rolling time window. Note, that for the correlation function in the cubic phase (for P=0, 8, 16 GPa) the x, y and z components of $C^\alpha(\tau)$ are degenerate and the lines are on top of each other.

# Supplemental References


[1] Zheyong Fan, Wei Chen, Ville Vierimaa, and Ari Harju. Efficient molecular dynamics simulations with many-body potentials on graphics processing units. *Computer Physics Communications*, 218:10–16, September 2017. doi: 10.1016/j.cpc.2017.05.003. URL `https://doi.org/10.1016/j.cpc.2017.05.003`.

[2] Zheyong Fan, Zezhu Zeng, Cunzhi Zhang, Yanzhou Wang, Keke Song, Haikuan Dong, Yue Chen, and Tapio Ala-Nissila. Neuroevolution machine learning potentials: Combining high accuracy and low cost in atomistic simulations and application to heat transport. *Physical Review B*, 104: 104309, Sep 2021. doi: 10.1103/PhysRevB.104.104309. URL `https://link.aps.org/doi/10.1103/PhysRevB.104.104309`.

[3] Zheyong Fan. Improving the accuracy of the neuroevolution machine learning potential for multi-component systems. *Journal of Physics: Condensed Matter*, 34(12):125902, jan 2022. doi: 10.1088/1361-648x/ac462b. URL `https://doi.org/10.1088/1361-648x/ac462b`.

[4] Daan Wierstra, Tom Schaul, Tobias Glasmachers, Yi Sun, Jan Peters, and Jürgen Schmidhuber. Natural evolution strategies. *Journal of Machine Learning Research*, 15(27):949–980, 2014. URL `http://jmlr.org/papers/v15/wierstra14a.html`.

[5] Erik Fransson, Julia Wiktor, and Paul Erhart. Phase transitions in inorganic halide perovskites from machine-learned potentials. *The Journal of Physical Chemistry C*, 127(28):13773–13781, July 2023. doi: 10.1021/acs.jpcc.3c01542. URL `https://doi.org/10.1021/acs.jpcc.3c01542`.

[6] A Togo and I Tanaka. First principles phonon calculations in materials science. *Scripta Materialia*, 108:1–5, November 2015. doi: 10.1016/j.scriptamat.2015.07.021.

[7] Erik Jedvik Granhed, Göran Wahnström, and Per Hyldgaard. $bazro_3$ stability under pressure: The role of nonlocal exchange and correlation. *Phys. Rev. B*, 101:224105, Jun 2020. doi: 10.1103/PhysRevB.101.224105. URL `https://link.aps.org/doi/10.1103/PhysRevB.101.224105`.

[8] Erik Jedvik Granhed. personal communication, 2023.

[9] Constance Toulouse, Danila Amoroso, Cong Xin, Philippe Veber, Monica Ciomaga Hatnean, Geetha Balakrishnan, Mario Maglione, Philippe Ghosez, Jens Kreisel, and Mael Guennou. Lattice dynamics and raman spectrum of $bazro_3$ single crystals. *Phys. Rev. B*, 100:134102, Oct 2019. doi: 10.1103/PhysRevB.100.134102. URL `https://link.aps.org/doi/10.1103/PhysRevB.100.134102`.

[10] Robert A. Evarestov. Hybrid density functional theory lcao calculations on phonons in $ba(ti,zr,hf)_3$. *Phys. Rev. B*, 83:014105, Jan 2011. doi: 10.1103/PhysRevB.83.014105. URL `https://link.aps.org/doi/10.1103/PhysRevB.83.014105`.

[11] D. Nuzhnyy, J. Petzelt, M. Savinov, T. Ostapchuk, V. Bovtun, M. Kempa, J. Hlinka, V. Buscaglia, M. T. Buscaglia, and P. Nanni. Broadband dielectric response of $ba(zr,ti)o_3$ ceramics: From incipient via relaxor and diffuse up to classical ferroelectric behavior. *Phys. Rev. B*, 86:014106, Jul 2012. doi: 10.1103/PhysRevB.86.014106. URL `https://link.aps.org/doi/10.1103/PhysRevB.86.014106`.

[12] Petter Rosander, Erik Fransson, Cosme Milesi-Brault, Constance Toulouse, Frédéric Bourdarot, Andrea Piovano, Alexei Bossak, Mael Guennou, and Göran Wahnström. Anharmonicity of the antiferrodistortive soft mode in barium zirconate $BaZrO_3$. *Phys. Rev. B*, 108:014309, Jul 2023. doi: 10.1103/PhysRevB.108.014309. URL `https://link.aps.org/doi/10.1103/PhysRevB.108.014309`.

[13] Yusheng Zhao and Donald J. Weidner. Thermal expansion of $srzro_3$ and $bazro_3$ perovskites. *Physics and Chemistry of Minerals*, 18:294–30, 1991. doi: 10.1007/BF00200187.

[14] Fredrik Eriksson, Erik Fransson, and Paul Erhart. The Hiphive Package for the Extraction of High-Order Force Constants by Machine Learning. *Adv. Theory Simul.*, 2(5):1800184, 2019. ISSN 2513-0390. doi: 10.1002/adts.201800184.

[15] L.-M. Peng, G. Ren, S. L. Dudarev, and M. J. Whelan. Robust Parameterization of Elastic and Absorptive Electron Atomic Scattering Factors. *Acta Crystallographica Section A*, 52 (2):257–276, Mar 1996. doi: 10.1107/S0108767395014371. URL https://doi.org/10.1107/S0108767395014371.

[16] L.-M. Peng. Electron Scattering Factors of Ions and their Parameterization. *Acta Crystallographica Section A*, 54(4):481–485, Jul 1998. doi: 10.1107/S0108767398001901. URL https://doi.org/10.1107/S0108767398001901.
